# Supplementary material for: POPT: Physics-Informed Deep Learning for Phase-Only Positioning in Distributed MIMO
Source: arXiv:2609.31218 source file (2026-09-25)
Supplement: Supplementary file 1 [file supplemental_material_final.tex]

%\documentclass[lettersize,journal]{IEEEtran}
%\usepackage{amsmath,amsfonts,amssymb}
%\usepackage{bm}
%\usepackage{mathtools}
%\usepackage{algorithmic}
%\usepackage{algorithm}
%\usepackage{array}
%\usepackage[caption=false,font=normalsize,labelfont=sf,textfont=sf]{subfig}
%\usepackage{textcomp}
%\usepackage{stfloats}
%\usepackage{url}
%\usepackage{verbatim}
%\usepackage{graphicx}
%\usepackage{cite}
%\usepackage[acronym]{glossaries}
%\usepackage{booktabs}
%\usepackage{multirow}
%\usepackage[hidelinks]{hyperref}
%\usepackage{bibentry}
%\usepackage{xr-hyper}
%\usepackage{microtype}
%\usepackage{xcolor}



%\makeglossaries
%\input{acronyms}

%\begin{document}

\setcounter{equation}{0}
\renewcommand{\theequation}{S\arabic{equation}}

\noindent{\Large\textbf{Supplementary Material:\vspace{2mm}\\``\textls[-5]{POPT: Physics-Informed Deep Learning for Phase-Only Positioning in Distributed MIMO}''}}

%\section*{Appendix}\\CRLB and PEB Derivation}
\vspace{6pt}

In this supplementary material, we derive the \gls{fim} of the channel parameters in Section~\ref{sec:channel_parameter_fim} and the transformation matrix, which is used to compute the \gls{fim} of the \gls{ue} state, in Section~\ref{sec:transformation_matrix}. We also provide the detailed mathematical expressions of the transformer encoder operations deferred from Section~\ref{subsubsec:encoder} in Section~\ref{sec:transformer_encoder_operations}.

\section{Channel Parameter FIM}\label{sec:channel_parameter_fim}

Let $\veta = [\phi, \alpha_1, \ldots, \alpha_M, \theta_1, \ldots, \theta_M]^\top$ denote the unknown channel parameter vector, for which the \gls{fim} is computed as
\begin{equation}\label{eq:channel_fim}
[\vJ(\veta)]_{ij} = \frac{2}{\sigma_w^2} \sum_{m=1}^{M} \Re \left \{
\frac{\partial \bar{y}_m^*}{\partial \veta_i}
\frac{\partial \bar{y}_m}{\partial \veta_j} \right \}, \:
i,j \in \{1,\ldots,2M+1\},
\end{equation}
where $\bar{y}_m = \sqrt{P} \alpha_{m}\exp{\left(-\jmath (\theta_{m} + \phi)\right)}s$ denotes the noise-free received signal. The \gls{fim} can be block-partitioned as follows
\begin{equation}
\vJ(\veta)=
\begin{bmatrix}
J_{\phi\phi}          & \vJ_{\phi\valpha}          & \vJ_{\phi\vtheta}\\
\vJ_{\valpha\phi}     & \vJ_{\valpha\valpha}       & \vJ_{\valpha\vtheta}\\
\vJ_{\vtheta\phi}     & \vJ_{\vtheta\valpha}       & \vJ_{\vtheta\vtheta}
\end{bmatrix},
\label{eq:FIM_block_partition}
\end{equation}
where $\valpha=[\alpha_1,\ldots,\alpha_M]^\top$ and $\vtheta=[\theta_1,\ldots,\theta_M]^\top$. The partial derivatives of $\bar{y}_m$ with respect to the channel parameters are 
\begin{equation}
    \frac{\partial \bar{y}_m}{\partial \phi} = -\jmath \bar{y}_m, \quad
    \frac{\partial \bar{y}_m}{\partial \alpha_{m'}} = \frac{\bar{y}_m}{\alpha_{m'}}, \quad
    \frac{\partial \bar{y}_m}{\partial \theta_{m'}} = -\jmath \bar{y}_m,
\end{equation}
in which $m' = m$, and otherwise the partial derivatives are
\begin{equation}
    \frac{\partial \bar{y}_m}{\partial \alpha_{m'}} = 0, \quad
    \frac{\partial \bar{y}_m}{\partial \theta_{m'}} = 0, \quad
    \text{if} \quad m \neq m'.
\end{equation}
Plugging the partial derivatives into \eqref{eq:channel_fim}, the block diagonal elements of the \gls{fim} are given by
\begin{subequations}
 \begin{align}
    J_{\phi\phi} &= \sum_{m=1}^M \frac{2P}{\sigma_w^2}  \alpha_m^2, \\
    \vJ_{\valpha\valpha}  &= \frac{2P}{\sigma_w^2}\vI_{M \times M}, \\
    \vJ_{\vtheta\vtheta}  &= \frac{2P}{\sigma_w^2} \diag([\alpha_1^2,\ldots,\alpha_M^2]). \label{eq:Jthetatheta}
\end{align}   
\end{subequations}
Respectively, the cross-elements of the \gls{fim} are given by
\begin{equation}
    \vJ_{\phi\valpha} = \mathbf{0}_{1 \times M}, \quad
    \vJ_{\phi\vtheta}  = \frac{2P}{\sigma_w^2} \valpha_{\text{sq}}^{\top}, \quad
    \vJ_{\valpha\vtheta}  = \mathbf{0}_{M \times M}.
\end{equation}
% \begin{subequations}
% \begin{align}
%     J_{\phi\valpha} &= \mathbf{0}_{1 \times M}, \\
%     \vJ_{\phi\vtheta}  &= \frac{2P}{\sigma_w^2} (\valpha^2)^\top, \\
%     \vJ_{\valpha\vtheta}  &= \mathbf{0}_{M \times M}.
% \end{align}
% \end{subequations}

\section{Transformation Matrix}\label{sec:transformation_matrix}

Next, we derive the transformation matrix, defined as 
\begin{equation}
[\vH_\vx(\vtheta)]_{m}
= \frac{\partial \theta_m}{\partial \vx}, \quad
m\in\{1,\ldots,M\}.
\end{equation}
By utilizing the definition of complex logarithm $\log z = \ln{\vert z \vert} + \jmath \arg{z} \Leftrightarrow \arg{z} = \Im\left\{ \log z \right\}$, the $m^{\text{th}}$ row of the Jacobian matrix can be written as 
\begin{subequations}
\begin{align} \label{eq:phase_diff}
\!\!\! \frac{\partial \theta_m}{\partial \vx} \!&=\! \Im \left\{ \frac{1}{\bar{y}_m} \frac{\partial \bar{y}_m}{\partial \vx} \right\} \\ \label{eq:phase_diff2}
&= \! \Im \left\{\frac{\sum_{i=1}^2 \! \left( \frac{\partial \alpha_m^{(i)}}{\partial \vx} \!-\! \jmath \alpha_m^{(i)} \frac{\partial \theta_m^{(i)}}{\partial \vx} \right)\exp(-\jmath\theta_m^{(i)}) }{\sum_{i=1}^2 h_m^{(i)}(\vx)}\right\},
\end{align}
\end{subequations}
where $\bar{y}_m = \sqrt{P}\big(h_m^{(1)}(\vx) + h_m^{(2)}(\vx) \big) \exp{(-\jmath\phi)}s$ is the received signal without noise.

The partial derivatives for the amplitude and phase of the LOS path can be straightforwardly obtained as
\begin{subequations}
\begin{align}
\frac{\partial \alpha_m^{(1)}}{\partial \vx} &= \frac{\lambda}{4\pi} \frac{\vdeltam^\top}{\Vert \vdeltam \Vert^3} \text{ and} \\
\frac{\partial \theta_m^{(1)}}{\partial \vx} &= -\frac{2\pi}{\lambda} \frac{\vdeltam^\top}{\Vert \vdeltam \Vert},
\end{align}
\end{subequations}
respectively, where $\vdeltam = \vp_m-\vx$. Furthermore, regarding the ground-reflected path, the corresponding partial derivatives of the amplitude and phase are given as
\begin{subequations}
\begin{align}
\frac{\partial \alpha_m^{(2)}}{\partial \vx} &= \frac{\lambda}{4\pi \Vert \vdeltamtilde \Vert} \left(\frac{\vert \Gamma_m(\vx)\vert \vdeltamtilde^\top}{\Vert \vdeltamtilde \Vert^2} + \frac{\partial \vert \Gamma_m(\vx)\vert}{\partial \vx}\right) \text{  and} \\
\frac{\partial \theta_m^{(2)}}{\partial \vx} &= -\frac{2\pi}{\lambda} \frac{\vdeltamtilde^\top}{\Vert \vdeltamtilde \Vert} - \frac{\partial \angle \Gamma_m(\vx)}{\partial \vx},
\end{align}
\end{subequations}
where $\vdeltamtilde = \tilde{\vp}_m-\vx$, and $\Gamma_m(\vx)$ is the reflection coefficient.

Considering the complex logarithm definition, used in \eqref{eq:phase_diff}, while exploiting the identities $\vert z \vert = \sqrt{z z^*}$ and $z + z^* = 2\Re\left\{ z \right\}$, the partial derivatives for the amplitude and phase of the reflection coefficient can be formulated as
\begin{subequations}
\begin{align}
\frac{\partial \vert \Gamma_m(\vx) \vert}{\partial \vx} &= \Re \left\{\frac{\Gamma_m^*(\vx)}{\vert \Gamma_m(\vx) \vert} \frac{\partial \Gamma_m(\vx)}{\partial \vx} \right\}\text{ and} \\
\frac{\partial \angle \Gamma_m(\vx)}{\partial \vx} &= \Im \left\{\frac{1}{\Gamma_m(\vx)} \frac{\partial \Gamma_m(\vx)}{\partial \vx} \right\},
\end{align}
\end{subequations}
respectively. After some algebraic manipulations, the complex-valued partial derivative of the reflection coefficient can be written as
\begin{align}
\frac{\partial \Gamma_m(\vx)}{\partial \vx} = \frac{2(1-\varepsilon_r)\sin(\gamma_m(\vx))}{\zeta(\vx)(\cos(\gamma_m(\vx)) + \zeta(\vx))^2} \frac{\partial \gamma_m(\vx)}{\partial \vx},
\end{align}
where %$\rho(\vx) = \cos(\gamma_m(\vx))$ and 
$\zeta(\vx) = \sqrt{\varepsilon_r - \sin^2(\gamma_m(\vx))}$. Furthermore, the partial derivative of the reflection angle reads
\begin{equation}
\frac{\partial \gamma_m(\vx)}{\partial \vx}
= -\frac{(z_m+z_{\textrm{ue}})\vdeltamtilde^\top + \left(d_m^{(2)}\right)^2 \mathbf{e}_3^\top}{\left(d_m^{(2)}\right)^3 \sqrt{1-\cos^2(\gamma_m(\vx))}},
%\left( \frac{z_{\textrm{ue}} + z_m}{d_m^{(2)}} \right)^2}}
\end{equation}
where $\mathbf{e}_3 = [0,0,1]^\top$.

% \begin{subequations}
% \begin{align}
%     \Gamma_m(\vx) &= \frac{\cos(\gamma_m(\vx)) - \sqrt{\varepsilon - \sin^2(\gamma_m(\vx))}}{\cos(\gamma_m(\vx)) + \sqrt{\varepsilon - \sin^2(\gamma_m(\vx))}} \\
%     &= \frac{\rho(\vx) - \zeta(\vx)}{\rho(\vx) + \zeta(\vx)}
% \end{align}
% \end{subequations}

%$\gamma_m(\vx) = \acos \left( \frac{z_{\textrm{ue}} + z_m}{d_m^{(2)}} \right)$


\section{Transformer Encoder Operations}\label{sec:transformer_encoder_operations}
The proposed encoder comprises $N_{\mathrm{enc}}$ stacked transformer encoder blocks that iteratively refine the token representations. Given the input representation $\mathbf{H}^{(0)}$ in \eqref{eq:final_popt_input}, the $q$-th encoder block, for $q\in\{1,\ldots,N_{\mathrm{enc}}\}$, adopts a pre-norm architecture expressed as


\begin{align}
\mathbf{Z}^{(q)} &= \mathrm{LN}\!\left(\mathbf{H}^{(q-1)}\right), \label{eq:enc_ln1}\\
\tilde{\mathbf{H}}^{(q)} &= \mathbf{H}^{(q-1)} + \mathrm{MHA}\!\left(\mathbf{Z}^{(q)}\right), \label{eq:enc_msa}\\
\mathbf{U}^{(q)} &= \mathrm{LN}\!\left(\tilde{\mathbf{H}}^{(q)}\right), \label{eq:enc_ln2}\\
\mathbf{H}^{(q)} &= \tilde{\mathbf{H}}^{(q)} + \mathrm{MLP}\!\left(\mathbf{U}^{(q)}\right), \label{eq:enc_ffn}
\end{align}
where the residual connections in \eqref{eq:enc_msa} and \eqref{eq:enc_ffn} maintain stable optimization by facilitating gradient propagation. \gls{ln} is defined for any vector $\mathbf{x}'$ as
\begin{equation}
\mathrm{LN}(\mathbf{x}')
=
\boldsymbol{\gamma}\odot
\frac{\mathbf{x}'-\mu(\mathbf{x}')}{\sqrt{\sigma^2(\mathbf{x}')+\epsilon}}
+\boldsymbol{\beta},
\end{equation}
where $\mu(\mathbf{x}')$ and $\sigma^2(\mathbf{x}')$ are the mean and variance of the entries of $\mathbf{x}'$, respectively, $\epsilon>0$ is a small constant, and $\boldsymbol{\gamma}$ and $\boldsymbol{\beta}$ are learnable vectors. In \eqref{eq:enc_ln1} and \eqref{eq:enc_ln2}, \gls{ln} is applied token-wise (row-wise) independently.

The \gls{mha} module computes queries, keys, and values through learned linear projections and, through its multi-head structure, allows the model to capture relationships in multiple representation subspaces. For head $h\in\{1,\ldots,N_{\mathrm{head}}\}$, the projections are
\begin{align}
\mathbf{Q}_{h}^{(q)} &= \mathbf{Z}^{(q)}\mathbf{W}_{Q,h}^{(q)}, \label{eq:Q_proj}\\
\mathbf{K}_{h}^{(q)} &= \mathbf{Z}^{(q)}\mathbf{W}_{K,h}^{(q)}, \label{eq:K_proj}\\
\mathbf{V}_{h}^{(q)} &= \mathbf{Z}^{(q)}\mathbf{W}_{V,h}^{(q)}, \label{eq:V_proj}
\end{align}
where
$\mathbf{W}_{Q,h}^{(q)},\mathbf{W}_{K,h}^{(q)},\mathbf{W}_{V,h}^{(q)}\in\mathbb{R}^{D_{\mathrm{emb}}\times d_h}$
are learnable weight matrices and $d_h=D_{\mathrm{emb}}/N_{\mathrm{head}}$ denotes the dimension of each attention head. The head output is computed using scaled dot-product attention as
\begin{equation}\label{eq:att_dot_prof}
\mathbf{A}_{h}^{(q)}=
\mathrm{softmax}\!\left(\frac{\mathbf{Q}_{h}^{(q)}\left(\mathbf{K}_{h}^{(q)}\right)^{\top}}{\sqrt{d_h}}\right)\mathbf{V}_{h}^{(q)}
\in\mathbb{R}^{M\times d_h},
\end{equation}
where $\mathrm{softmax}(\cdot)$ exponentiates each entry and normalizes each row independently. The scaling factor $1/\sqrt{d_h}$ prevents the inner products from growing excessively. Finally, the head outputs are concatenated and linearly transformed as
\begin{equation}\label{eq:mha}
\mathrm{MHA}\!\left(\mathbf{Z}^{(q)}\right)=
\!\left[\mathbf{A}_{1}^{(q)},\ldots,\mathbf{A}_{N_{\mathrm{head}}}^{(q)}\right]\mathbf{W}_{O}^{(q)},
\end{equation}
where $\mathbf{W}_{O}^{(q)}\in\mathbb{R}^{D_{\mathrm{emb}}\times D_{\mathrm{emb}}}$ is a learnable matrix.

The \gls{mlp} block in \eqref{eq:enc_ffn} is applied independently to each
row (token) of $\mathbf{U}^{(q)}$, and consists of two fully connected layers
with \gls{gelu} activation. For a row vector $\mathbf{u}\in\mathbb{R}^{D_{\mathrm{emb}}}$
corresponding to a single token, the MLP is defined as
\begin{equation}\label{eq:popt_mlp}
\mathrm{MLP}(\mathbf{u})=
\mathrm{GELU}\!\left(\mathbf{u}\mathbf{W}_{1}^{(q)}+\mathbf{b}_{1}^{(q)}\right)\mathbf{W}_{2}^{(q)}+\mathbf{b}_{2}^{(q)},
\end{equation}
where $D_{\mathrm{ff}}$ denotes the feed-forward hidden dimension, and
$\mathbf{W}_{1}^{(q)}\in\mathbb{R}^{D_{\mathrm{emb}}\times D_{\mathrm{ff}}}$
and $\mathbf{W}_{2}^{(q)}\in\mathbb{R}^{D_{\mathrm{ff}}\times D_{\mathrm{emb}}}$
are learnable weight matrices, while
$\mathbf{b}_{1}^{(q)}\in\mathbb{R}^{D_{\mathrm{ff}}}$ and
$\mathbf{b}_{2}^{(q)}\in\mathbb{R}^{D_{\mathrm{emb}}}$ are learnable bias vectors. After $N_{\mathrm{enc}}$ layers, the encoder output is $\mathbf{H}^{(N_{\mathrm{enc}})}\in\mathbb{R}^{M\times D_{\mathrm{emb}}}$, which is then passed to the Output Head described in the main text.


\section{Complexity Derivations for Benchmark Methods}\label{sec:benchmark_complexity}
The benchmark \gls{mlp} consists of seven hidden layers with widths $A,\,2A,\,4A,\,8A,\,4A,\,2A,$ and $A$, where $A=128$ as in~\cite{11275391}. The input dimension of the benchmark \gls{mlp} is $M-1$, corresponding to the differential phase measurements. Hence, the inference cost includes the input-to-hidden layer, the six hidden-to-hidden fully connected layers, and the output layer. The resulting complexity therefore scales as $\mathcal{O}_{\text{MLP}}=\mathcal{O}\!\left((M-1)A + A^2\right)$,
\begin{comment}
    \begin{equation}\label{eq:mlp_bigO}
\mathcal{O}_{\text{MLP}}=\mathcal{O}\!\left((M-1)A + A^2\right).
\end{equation}
\end{comment}
and the total number of \glspl{flop} can be approximated as~\cite{11275391} $\mathcal{F}_{\text{MLP}} \approx 168A^2 = 2.75\times 10^6$.
\begin{comment}
    \begin{equation}\label{eq:mlp_flop}
\mathcal{F}_{\text{MLP}} \approx 168A^2 = 2.75\times 10^6.
\end{equation}
\end{comment}

The \gls{hi} benchmark in~\cite{11274977} consists of an \gls{mlp}-based differential ambiguity estimator followed by a gradient-based solver. Following the parameterization in~\cite{11274977}, the total inference \gls{flop} count can be written as $\mathcal{F}_{\mathrm{HI}} \approx 7.5\times 10^4\,M + 256\,Q + 1.92\times 10^5$, where $Q$ denotes the total number of output classes of the ambiguity estimator. Since $Q$ grows linearly with $M$, the overall complexity becomes $\mathcal{O}(M)$.
\begin{comment}
    \begin{equation}\label{eq:hi_bigO}
\mathcal{O}(M).
\end{equation}
\end{comment}

\begin{comment}
    \begin{equation}\label{eq:hi_flop}
\mathcal{F}_{\mathrm{HI}}
\approx
7.5\times 10^4\,M + 256\,Q + 1.92\times 10^5,
\end{equation}
\end{comment}



%\bibliographystyle{IEEEtran}
%\nobibliography{references}

%\end{document}
